# Supplementary material for: Editing Factual Knowledge and Explanatory Ability of Medical Large Language Models
Source: arXiv:2402.18099 source file (2024-09-23)
Supplement: Supplementary file 1 [file 08_appendix.tex]

\section{Data Samples}\label{app:DataSamples}
We provide data samples for the MedCF and MedFE datasets in Figure \ref{fig:medcf_datacase} and \ref{fig:medfe_datacase}, comprising of the knowledge that requires editing, rephrase knowledge, and irrelevant knowledge obtained through our proposed methodology in Section \ref{sec:ConstructingLocalityEvaluation}.

\begin{figure*}[t]
\begin{center}
\includegraphics[scale=0.45]{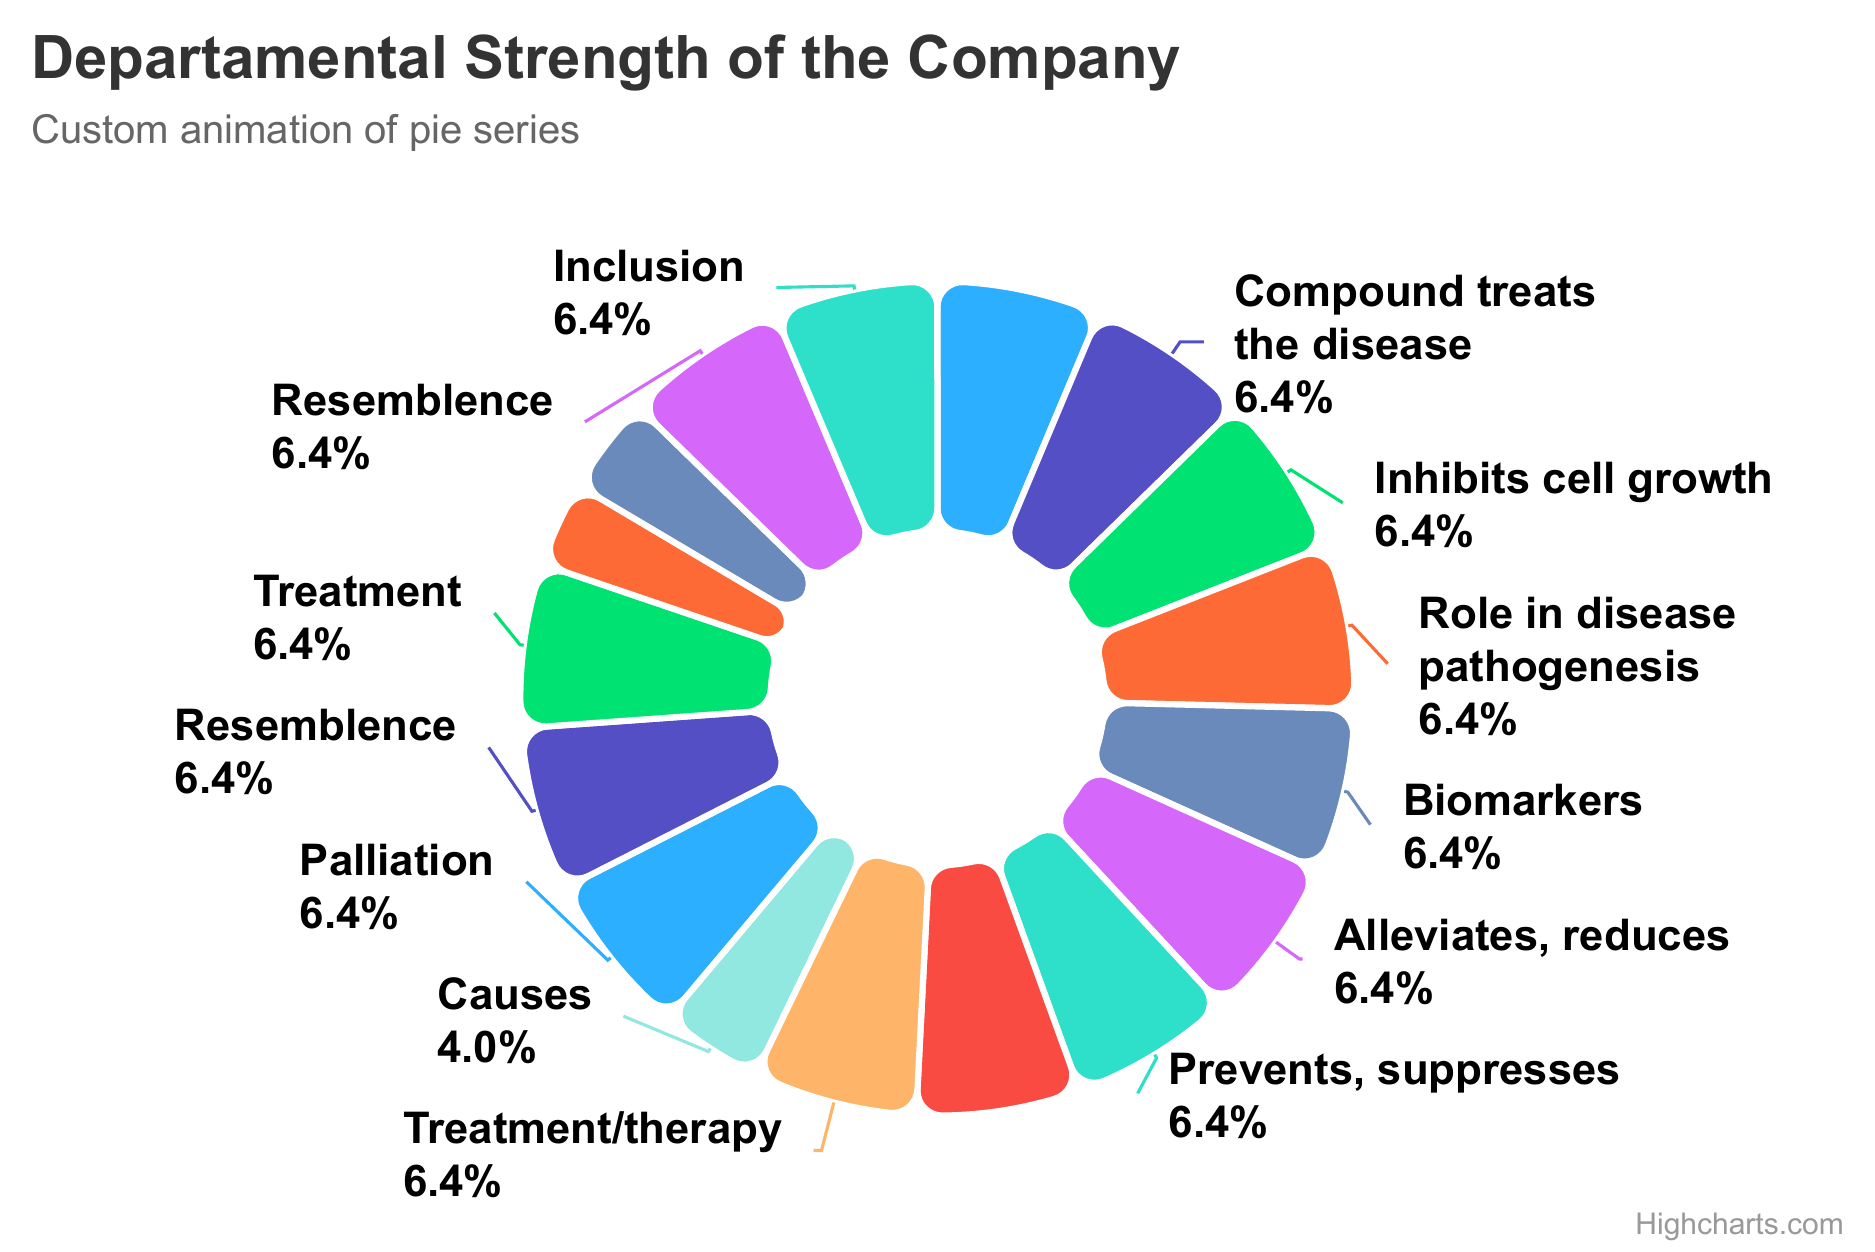}
\caption{A sample of the MedCF dataset.}
\label{fig:medcf_datacase}
\end{center}
\end{figure*}

\begin{figure*}[t]
\begin{center}
\includegraphics[scale=0.45]{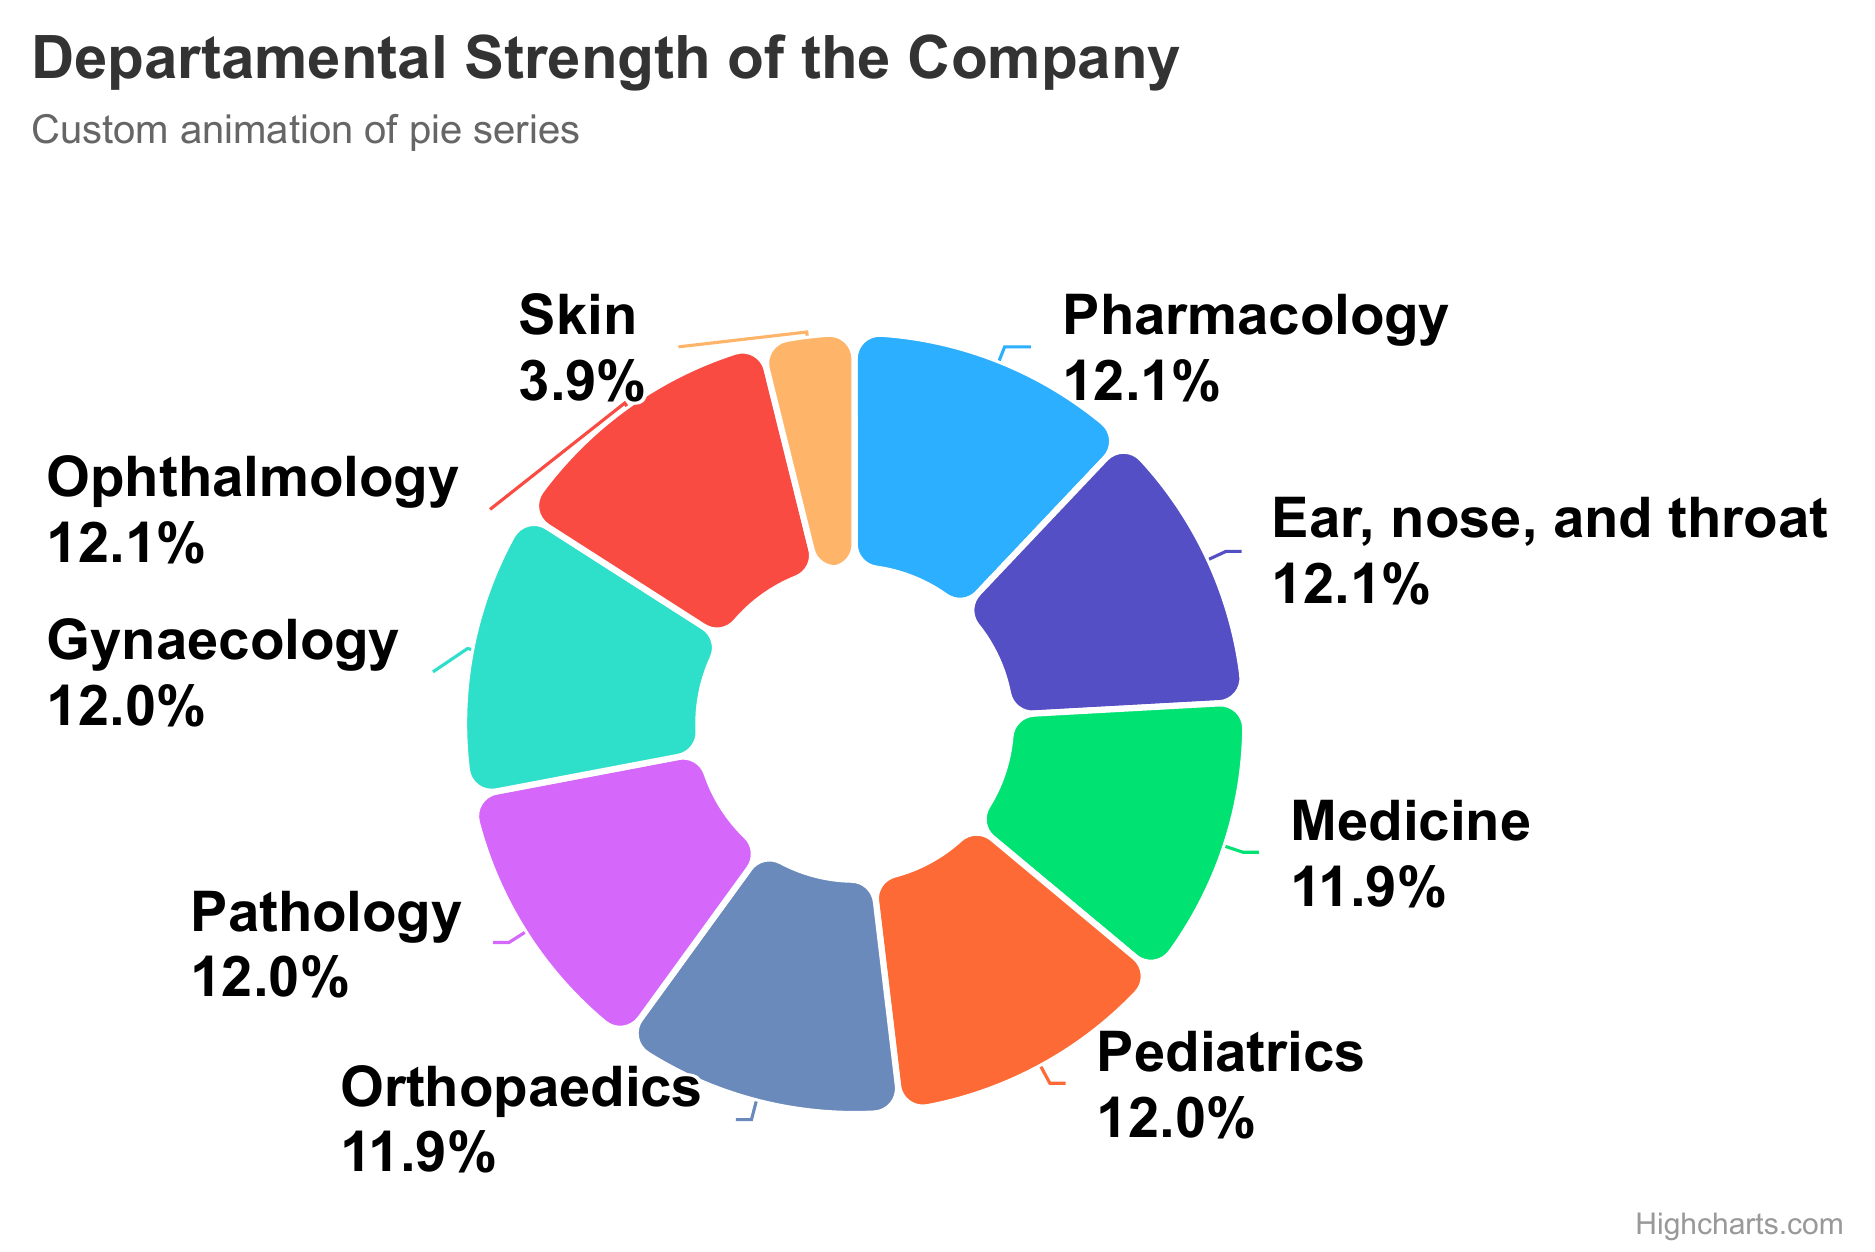} 
\caption{A sample of the MedFE dataset.}
\label{fig:medfe_datacase}
\end{center}
\end{figure*}

\section{Case of Causal Tracing}\label{app:CaseCausalTracing}
In this section, we showcase heatmaps illustrating individual instances of Causal tracing from the MedCF and MedFE datasets on ChatDoctor network parameters (including Attn and MLP networks) in Figure \ref{fig:medcf_datacase} and \ref{fig:medfe_datacase}. These heatmaps provide a visual representation of the Causal tracing, allowing us to visually understand how the model makes decisions and pinpoint areas that can be enhanced. By examining these heatmaps, we can extract valuable information about how the model makes decisions and establish factual connections with particular neuron activations \cite{rome}. 

\begin{figure*}[t]
\centering
\includegraphics[width=0.8\columnwidth]{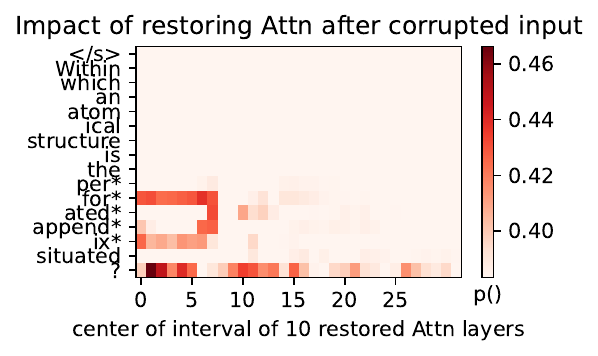}
\includegraphics[width=0.8\columnwidth]{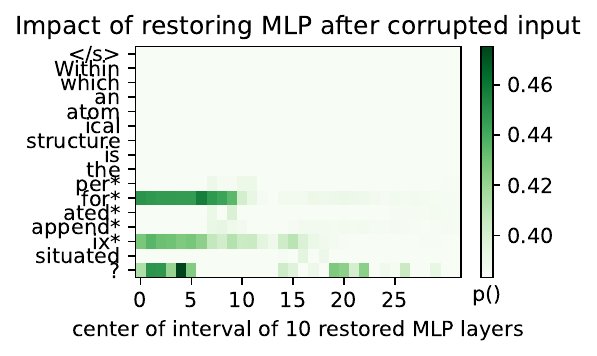}
\includegraphics[width=0.8\columnwidth]{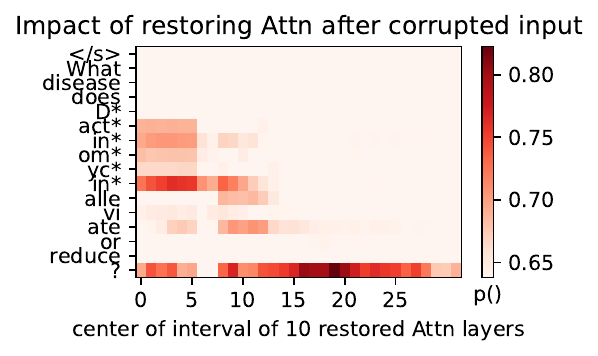}
\includegraphics[width=0.8\columnwidth]{img/MedCF_10_attn.pdf}
\caption{Case of Causal tracing on the MedCF dataset.
}
\label{fig:MedCFCausaltracing}
\end{figure*}
\begin{figure*}[t]
\centering
\includegraphics[width=0.8\columnwidth]{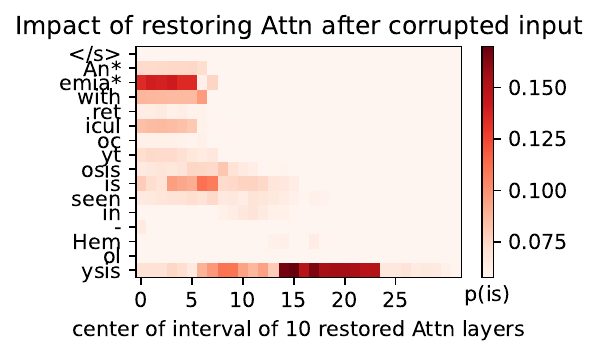}
\includegraphics[width=0.8\columnwidth]{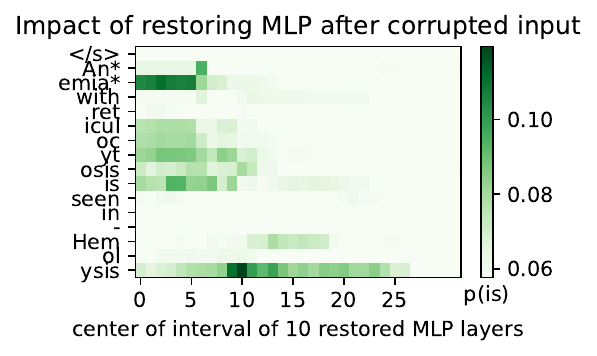}
\includegraphics[width=0.8\columnwidth]{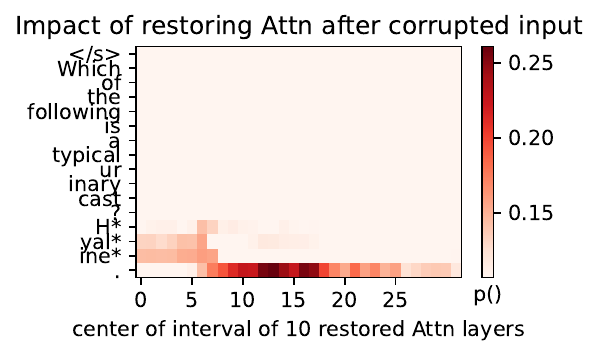}
\includegraphics[width=0.8\columnwidth]{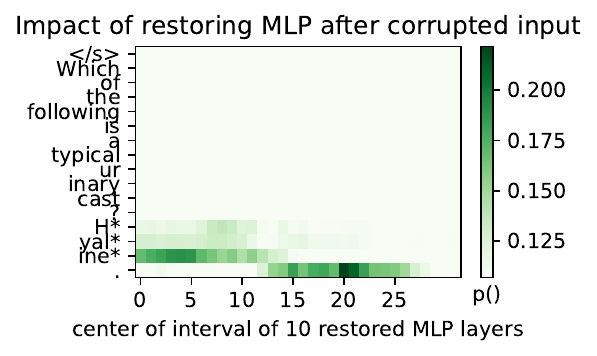}
\caption{Case of Causal tracing on the MedFE dataset.
}
\label{fig:MedFECausaltracing}
\end{figure*}
